# Supplementary material for: Boltzmann approach to collective motion via nonlocal visual interaction
Source: arXiv:2408.09917 ancillary file (2025-03-15)
Supplement: Supplementary file 1 [file Supplemental_Material.pdf]

# Supplemental Material for “Boltzmann approach to collective motion via non-local visual interaction”

Susumu Ito, and Nariya Uchida\*

*Department of Physics, Tohoku University, Sendai, 980-8578, Japan*

(Dated: March 14, 2025)

## CONTENTS

|                                                                        |   |
|------------------------------------------------------------------------|---|
| I. Derivation of $\mathcal{D}(R)$                                      | 2 |
| II. Definition of the parameters                                       | 3 |
| III. An alternative form of $K(\psi)$                                  | 4 |
| IV. Scaling law for the polar order parameter                          | 5 |
| V. Correspondence with the local collision model as the singular limit | 6 |
| References                                                             | 7 |

---

\* uchida@cmpt.phys.tohoku.ac.jp

# I. DERIVATION OF $\mathcal{D}(R)$

Here, we derive the average arc length occupied by an agent  $\mathcal{D}(R)$  inside the angle  $\Phi$ . We introduce the body length (the diameter of an agent)  $D$  and the azimuth  $\phi \in [-\frac{\Phi}{2}, \frac{\Phi}{2}]$ . The averaged body length inside the angular region  $\Phi$  which is sufficiently small is defined as

$$\mathcal{D}(R) = \frac{1}{\Phi} \int_{-\frac{\Phi}{2}}^{\frac{\Phi}{2}} d\phi \tilde{D}(R, \phi), \quad (\text{S1})$$

where  $\tilde{D}(R, \phi)$  represents the visible arc length of an agent whose center at  $(R, \phi)$  inside the angle  $\Phi$  (see also Fig. S1). There are the following cases depending on  $R$ .

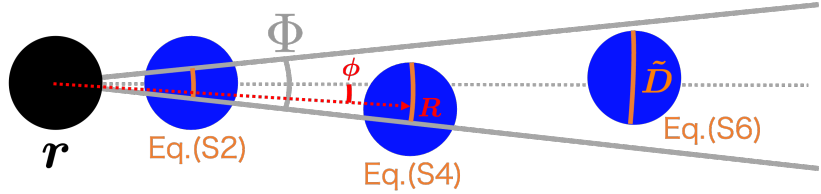

FIG. S1. Schematic illustration of  $\tilde{D}$  corresponding to Eq. (S2), (S4), (S6).

- In the case of  $R < \frac{D}{2\Phi}$ .

The angular region  $\Phi$  is filled by an agent at any azimuth  $\phi$ , and therefore

$$\tilde{D}(R, \phi) = R\Phi, \quad (\text{S2})$$

and we obtain

$$\mathcal{D}(R) = R\Phi. \quad (\text{S3})$$

- In the case of  $\frac{D}{2\Phi} < R < \frac{D}{\Phi}$ .

The angular region  $\Phi$  is filled by an agent only at  $\frac{\Phi}{2} - \frac{D}{2R} < \phi < -\frac{\Phi}{2} + \frac{D}{2R}$ . On the other hand, there is the interstice inside  $\Phi$  at the other region of  $\phi$ . By the linear interpolation,  $\tilde{D}(R, \phi)$  takes the form

$$\tilde{D}(R, \phi) = \begin{cases} R(\phi + \frac{\Phi}{2} + \frac{D}{2R}) & [\phi < \frac{\Phi}{2} - \frac{D}{2R}], \\ R\Phi & [\frac{\Phi}{2} - \frac{D}{2R} < \phi < -\frac{\Phi}{2} + \frac{D}{2R}], \\ R(-\phi + \frac{\Phi}{2} + \frac{D}{2R}) & [\phi > -\frac{\Phi}{2} + \frac{D}{2R}], \end{cases} \quad (\text{S4})$$

and then we obtain

$$\mathcal{D}(R) = D \left( 1 - \frac{D}{4R\Phi} \right). \quad (\text{S5})$$

- In the case of  $R > \frac{D}{\Phi}$ .

The angular region  $\Phi$  is not filled by an agent at any azimuth  $\phi$ , and there is the interstices at both side of an agent when  $-\frac{\Phi}{2} + \frac{D}{2R} < \phi < \frac{\Phi}{2} - \frac{D}{2R}$ . Therefore,

$$\tilde{D}(R, \phi) = \begin{cases} R(\phi + \frac{\Phi}{2} + \frac{D}{2R}) & [\phi < -\frac{\Phi}{2} + \frac{D}{2R}], \\ D & [-\frac{\Phi}{2} + \frac{D}{2R} < \phi < \frac{\Phi}{2} - \frac{D}{2R}], \\ R(-\phi + \frac{\Phi}{2} + \frac{D}{2R}) & [\phi > \frac{\Phi}{2} - \frac{D}{2R}], \end{cases} \quad (\text{S6})$$

and we obtain

$$\mathcal{D}(R) = D \left( 1 - \frac{D}{4R\Phi} \right), \quad (\text{S7})$$

which is the same form as Eq. (S5).

Finally, we obtain

$$\mathcal{D}(R) = \begin{cases} R\Phi & [R < \frac{D}{2\Phi}] , \\ D \left( 1 - \frac{D}{4R\Phi} \right) & [R > \frac{D}{2\Phi}] , \end{cases} \quad (\text{S8})$$

which is identical to Eq. (7) by  $R_D = D/(2\Phi)$ .

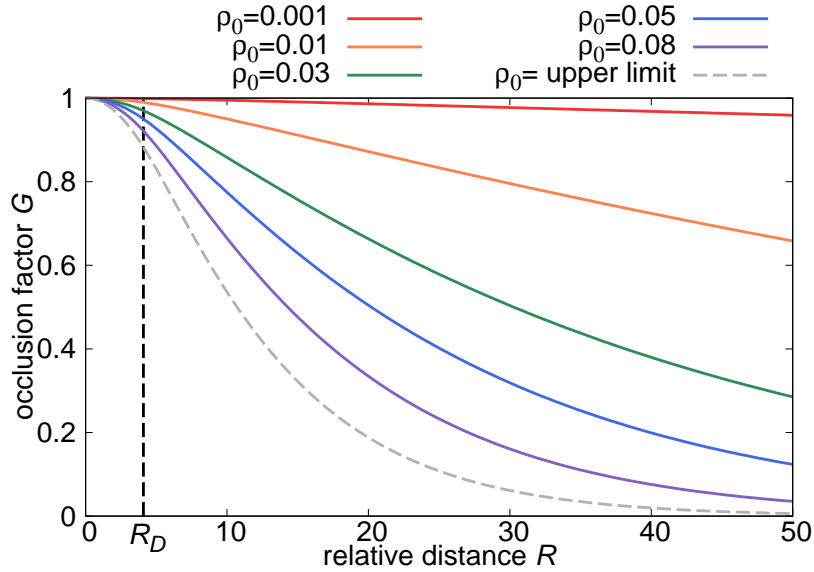

FIG. S2. The occlusion factor  $G$  as a function of the relative distance  $R$  for the uniform density  $\rho_0$ . The solid lines represent the occlusion factor with  $\rho_0 = 0.001, 0.01, 0.03, 0.05, 0.08$ . The gray dashed line is the occlusion factor with the upper limit density  $\rho_0 = \Phi/D^2$ . The vertical dashed line corresponds to  $R = R_D$  in Eq. (7). The parameters are  $D = 1$ ,  $\Phi = 7^\circ$  which are the same as that in Fig. 3.

## II. DEFINITION OF THE PARAMETERS

Here, we show the definition of parameters and the adopted value in our model. It is possible to determine the parameter values for various organisms by performing the appropriate experiments. Here we adopt the values for fish that have been already well studied experimentally to ensure that our results are reasonable. Note that our analytical results on the qualitative properties of the phase transition does not depend on the appropriate choice of parameter values.

- The diameter corresponds to a body length:  $D = 1$  BL (BL is the abbreviation of body length).
- Zebrafish (*Danio rerio*) changes the direction of motion with  $\sim 2.5$  Hz which corresponds to the frequency of tail beat [3]. In addition, many species of fish takes  $\sim 2$  Hz for the frequency of tail beat with the steady swimming speed 1 BL/s [4, 5]. Thus, we get  $s = 2 \text{ s}^{-1}$ .
- The probability distribution of direction change  $p(\theta)$  is the von Mises distribution for zebrafish with the sharpness  $\kappa \sim 6.3$  [3], and then we set  $\kappa = 6$ . In addition, the previous agent-based model [3] set  $\hat{\kappa} = 20$ , and we also

adopt this value. In this case, the Fourier component satisfies  $2\pi\hat{p}_1 = I_1(\hat{\kappa})/I_0(\hat{\kappa}) \simeq 0.97 > 3/4$  in which the phase transition can occur. (See Sect. IV. E. for the details.)

- For zebrafish and golden shiner (*Notemigonus crysoleucas*), the limit distance is  $\sim 8\text{--}39$  BL at which an individual can visually recognize a distant neighbor [1]. Converting these distance to the angular diameter yields  $1.5\text{--}7^\circ$ . We adopt  $\Phi = 7^\circ$ , and therefore  $R_D = D/(2\Phi) = 90/(7\pi)$  BL.
- For rummy-nose tetra (*Hemigrammus rhodostomus*), the characteristic length of orientational interaction is estimated as at least  $\sim 8$  BL [2]. We set  $R_0 = 10$  BL, which is comparable to the typical distance of a neighbor  $r$  near the upper limit density  $\rho_0 = \Phi/D^2$ . In other words, the occlusion factor  $G$  is comparable to the intrinsic factor  $B$  as the density approaches to the upper limit.

The length and time unit are rescaled by the body length  $D$  (the diameter of an agent) and 1 second, respectively. Then we get the parameter value in the main text, and the region of the density in the limit of application of the model is  $\rho_0 \ll 0.12$  (see Fig. 3).

### III. AN ALTERNATIVE FORM OF $K(\psi)$

We define  $K(\psi) = \sqrt{2}|\sin \psi|$  in this paper based on the biological consideration, however we show that similar properties of the phase transition can be obtained using a different function  $K(\psi)$ . For example, we take  $K(\psi) = \sqrt{2(1 - \cos \psi)}$  which is used in the local collision model [6]. It is derived from the relative velocity between an agent with  $\theta$  and another agent with  $\theta'$ :  $|\mathbf{e}(\theta') - \mathbf{e}(\theta)| = |(\cos \theta' - \cos \theta, \sin \theta' - \sin \theta)| = \sqrt{2(1 - \cos(\theta' - \theta))}$ . In other words, an agent easily reacts to a neighbor with the relative angle  $\psi = \pm\pi$ . In this case,

$$K_k = \frac{4}{\pi} \frac{1}{1 - (2k)^2}, \quad (\text{S9})$$

and we substitute this into Eq. (A.36) and obtain

$$\text{Re } \Lambda_k(\mathbf{q}) = s(1 - 2\pi p_k) + 8c\mathcal{I}\overline{f_0}W_k(\mathbf{q}). \quad (\text{S10})$$

$$W_k(\mathbf{q}) := 1 + \hat{\mathcal{I}}(\mathbf{q}) \frac{1}{1 - (2k)^2} - (2\pi\hat{p}_k) \left(1 + \hat{\mathcal{I}}(\mathbf{q})\right) \left( \frac{\delta_{k,\text{even}}}{1 - k^2} + \frac{1}{2}\delta_{k,\pm 1} - \frac{(-1)^{\frac{k-1}{2}}k - 1}{1 - k^2} \delta_{k,\{\pm 3, \pm 5, \dots\}} \right). \quad (\text{S11})$$

- In the case of  $k = \pm 1$ ,  $W_{\pm 1}(\mathbf{q}) = 1 - \frac{1}{3}\hat{\mathcal{I}}(\mathbf{q}) - \frac{1}{2} \times (2\pi\hat{p}_k) \left(1 + \hat{\mathcal{I}}(\mathbf{q})\right)$ .
- In the case of  $k = \text{even}$ ,  $W_k(\mathbf{q}) = 1 - \frac{1}{(2k)^2 - 1}\hat{\mathcal{I}}(\mathbf{q}) + \frac{1}{k^2 - 1}(2\pi\hat{p}_k) \left(1 + \hat{\mathcal{I}}(\mathbf{q})\right) > 0$ .
- In the case of  $k = \text{odd}$  and  $k \neq \pm 1$ ,

$$W_k(\mathbf{q}) = 1 - \frac{1}{(2k)^2 - 1}\hat{\mathcal{I}}(\mathbf{q}) - \frac{(-1)^{\frac{k-1}{2}}k - 1}{k^2 - 1}(2\pi\hat{p}_k) \left(1 + \hat{\mathcal{I}}(\mathbf{q})\right) \geq 1 - \frac{1}{(2k)^2 - 1}\hat{\mathcal{I}}(\mathbf{q}) - \frac{1}{|k| + 1}(2\pi\hat{p}_k) \left(1 + \hat{\mathcal{I}}(\mathbf{q})\right) > 0. \quad (\text{S12})$$

Therefore, in this case also,

$$\text{Re } \Lambda_1(\mathbf{q}) = s(1 - 2\pi p_1) - 8c\mathcal{I}\overline{f_0} \left\{ \frac{1}{3}\hat{\mathcal{I}}(\mathbf{q}) + \frac{1}{2} \times (2\pi\hat{p}_1) \left(1 + \hat{\mathcal{I}}(\mathbf{q})\right) - 1 \right\}, \quad (\text{S13})$$

only becomes negative and the phase transition occurs. In particular,

$$\text{Re } \Lambda_1(\mathbf{0}) = s(1 - 2\pi p_1) - 8c\mathcal{I}\overline{f_0} \left( 2\pi\hat{p}_1 - \frac{2}{3} \right) \quad (\text{S14})$$

shows that the transition occurs in the case of  $2\pi\hat{p}_1 > \frac{2}{3}$ . Therefore, the choice of  $K(\psi)$  is qualitatively unimportant unless  $K(\psi)$  is a constant.

#### IV. SCALING LAW FOR THE POLAR ORDER PARAMETER

Here, we show the scaling law of polar order parameter  $P$  with respect to  $c - c_{\text{tr}}$  when the advection term is absent. The reason why we can neglect the advection term in the vicinity of the transition point and for sufficiently small  $v_0$  is provided in the main text.

As mentioned before, the number density is uniform at the transition point, and we then consider the distribution function  $f(\theta) = \sum_k f_k e^{ik\theta}$  in the steady state. Note that, when we consider a finite two dimensional region  $L \times L$  with the periodic boundary condition, the ultra long wavelength mode ( $\mathbf{q} \simeq 0$ ) is truncated, and then the uniform number density is maintained near the transition point. In this case, the Boltzmann equation (Eq. (1)) becomes as follows by using the calculation techniques in Sect. IV.

$$0 = -s \sum_k f_k e^{ik\theta} + s \sum_k (2\pi p_k) f_k e^{ik\theta} - 2\pi c \mathcal{I} \sum_{k,k'} K_{k'} f_{k'} f_k e^{i(k+k')\theta} + 2\pi c \mathcal{I} \sum_{k,k',k''} (2\pi \hat{p}_k) K_{k'} f_{k''} f_{k-k''} \left( \delta_{k,-2(k'-k'')} + \frac{2}{\pi} \frac{(-1)^{k'-k''} (-1)^{\frac{k-1}{2}}}{k+2(k'-k'')} \delta_{k,\text{odd}} \right) e^{ik\theta}. \quad (\text{S15})$$

Furthermore, near the transition point, the local vector order parameter  $\mathbf{E} = \int_{-\pi}^{\pi} d\theta \mathbf{e}(\theta) f(\theta) / \rho_0$  is small and we define its magnitude as  $\epsilon \ll 1$ , and then  $f_k = \mathcal{O}(\epsilon^{|k|})$ . Therefore, we consider only the component  $f_0, f_{\pm 1}, f_{\pm 2}$  and truncate the hierarchy at  $\mathcal{O}(\epsilon^3)$  [6].

We multiply  $e^{-i\theta}$  with the both sides of Eq. (S15) and integrate in terms of  $\theta$ , and we obtain

$$0 = - \left\{ s(1 - 2\pi p_1) - 4\sqrt{2}c\mathcal{I}f_0 \left( \frac{4}{3} \times (2\pi \hat{p}_1) - 1 \right) \right\} f_1 - \frac{28\sqrt{2}}{15} c\mathcal{I}(2\pi \hat{p}_1) f_{-1} f_2 \quad (\text{S16})$$

where we use Eqs. (A.37), (A.39). Next, we multiply  $e^{-2i\theta}$  with the both sides of Eq. (S15) and integrate in terms of  $\theta$  to get

$$0 = - \left\{ s(1 - 2\pi p_2) + \frac{8\sqrt{2}}{3} c\mathcal{I}f_0 \right\} f_2 + 4\sqrt{2}c\mathcal{I}(2\pi \hat{p}_2) f_1^2 \quad (\text{S17})$$

and

$$f_2 = \frac{4\sqrt{2}c\mathcal{I}(2\pi \hat{p}_2)}{s(1 - 2\pi p_2) + \frac{8\sqrt{2}}{3} c\mathcal{I}f_0} f_1^2. \quad (\text{S18})$$

Therefore, from Eqs. (S16), (S18) and Eq. (A.42), we obtain

$$0 = 4\sqrt{2} \left( \frac{4}{3} \times (2\pi \hat{p}_1) - 1 \right) \mathcal{I}f_0 f_1 (c - c_{\text{tr}}) - \frac{28\sqrt{2}}{15} c\mathcal{I}(2\pi \hat{p}_1) \times \frac{4\sqrt{2}c\mathcal{I}(2\pi \hat{p}_2)}{s(1 - 2\pi p_2) + \frac{8\sqrt{2}}{3} c\mathcal{I}f_0} |f_1|^2 f_1 \quad (\text{S19})$$

( $f_{-1} = f_1^*$ ) and thus

$$|f_1|^2 = \frac{15 \left( \frac{4}{3} \times (2\pi \hat{p}_1) - 1 \right) \left( s(1 - 2\pi p_2) + \frac{8\sqrt{2}}{3} c_{\text{tr}} \mathcal{I}f_0 \right)}{28\sqrt{2}c_{\text{tr}}^2 \mathcal{I}f_0 (2\pi \hat{p}_1) (2\pi \hat{p}_2)} f_0^2 (c - c_{\text{tr}}) \quad (\text{S20})$$

where we replace  $c$  to  $c_{\text{tr}}$ , except for  $c - c_{\text{tr}}$ .

On the other hand, the polar order parameter is rewritten as

$$\begin{aligned} P &= |\mathbf{E}| \\ &= \frac{1}{\rho_0} \left| \int_{-\pi}^{\pi} d\theta \mathbf{e}(\theta) f(\theta) \right| \\ &= \frac{1}{\rho_0} \left| \int_{-\pi}^{\pi} d\theta \left( \frac{e^{i\theta} + e^{-i\theta}}{2}, \frac{e^{i\theta} - e^{-i\theta}}{2i} \right) (f_1 e^{i\theta} + f_{-1} e^{-i\theta}) \right| \\ &= \frac{2\pi}{\rho_0} |f_1|. \end{aligned} \quad (\text{S21})$$

Therefore, we obtain finally

$$P = \left\{ \frac{15 \left( \frac{4}{3} \times (2\pi\hat{p}_1) - 1 \right) \left( s(1 - 2\pi p_2) + \frac{8\sqrt{2}}{3} c_{\text{tr}} \mathcal{I} f_0 \right)}{28\sqrt{2} c_{\text{tr}}^2 \mathcal{I} f_0 (2\pi\hat{p}_1)(2\pi\hat{p}_2)} \right\}^{\frac{1}{2}} (c - c_{\text{tr}})^{\frac{1}{2}} := P_0(c_{\text{tr}})(c - c_{\text{tr}})^{\frac{1}{2}}. \quad (\text{S22})$$

See Fig. S3 for the map of the prefactor  $P_0(c_{\text{tr}})$ .

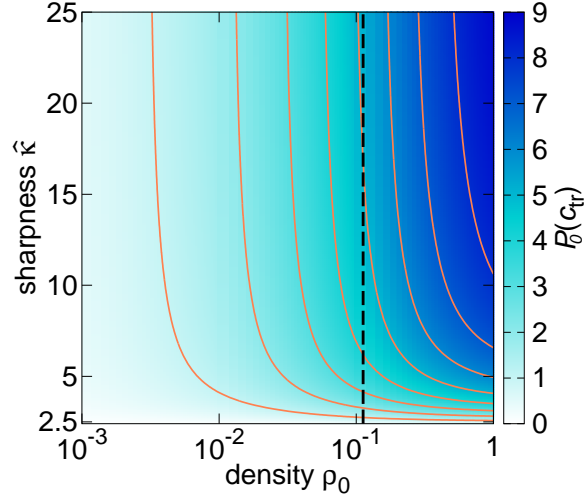

FIG. S3. The scaling prefactor  $P_0(c_{\text{tr}})$  as a function of  $\rho_0$  and  $\hat{\kappa}$  which is the sharpness parameter of  $\hat{p}(\theta)$ . The value of the parameter set is the same as that in Fig. 3, except for  $2.4 < \hat{\kappa} < 25$  ( $2\pi\hat{p}_1|_{\hat{\kappa}=2.4} \simeq 0.754 > 3/4$  is satisfied). The black dashed line represents that of the application condition of  $\rho_0$ . The orange contours correspond to  $P_0(c_{\text{tr}}) = 1, 2, \dots, 9$ .

## V. CORRESPONDENCE WITH THE LOCAL COLLISION MODEL AS THE SINGULAR LIMIT

Here, we consider the correspondence of our model with the local collision model.  $I_{\text{vis}}[f]$  is

$$\begin{aligned} I_{\text{vis}}[f] = & -c \int d^2\mathbf{r}' \int_{-\pi}^{\pi} d\theta' G(\mathbf{r}, \mathbf{r}' - \mathbf{r}, t) \exp\left(-\frac{|\mathbf{r}' - \mathbf{r}|^2}{2R_0^2}\right) K(\theta' - \theta) f(\mathbf{r}, \theta, t) f(\mathbf{r}', \theta', t) \\ & + c \int d^2\mathbf{r}' \int_{-\pi}^{\pi} d\theta_1 \int_{-\pi}^{\pi} d\theta_2 G(\mathbf{r}, \mathbf{r}' - \mathbf{r}, t) \exp\left(-\frac{|\mathbf{r}' - \mathbf{r}|^2}{2R_0^2}\right) K(\theta_2 - \theta_1) f(\mathbf{r}, \theta_1, t) f(\mathbf{r}', \theta_2, t) \hat{p}(\theta - \vartheta(\theta_1, \theta_2)). \end{aligned} \quad (\text{S23})$$

In order to obtain the local collision term

$$\begin{aligned} I_{\text{col}}[f] = & -c_{\text{col}} \int_{-\pi}^{\pi} d\theta' K(\theta' - \theta) f(\mathbf{r}, \theta, t) f(\mathbf{r}, \theta', t) \\ & + c_{\text{col}} \int_{-\pi}^{\pi} d\theta_1 \int_{-\pi}^{\pi} d\theta_2 K(\theta_2 - \theta_1) f(\mathbf{r}, \theta_1, t) f(\mathbf{r}, \theta_2, t) \hat{p}(\theta - \vartheta(\theta_1, \theta_2)) \end{aligned} \quad (\text{S24})$$

from  $I_{\text{vis}}[f]$ , where  $c_{\text{col}}$  is a rate of collision per unit time, the spatial dependence term  $\exp\left(-\frac{|\mathbf{r}' - \mathbf{r}|^2}{2R_0^2}\right)$  should become the Dirac delta function  $\delta(\mathbf{r}' - \mathbf{r})$ . Therefore, the rate  $c$  should be replaced by  $c = c_{\text{col}}/(2\pi R_0^2)$ , and  $\exp\left(-\frac{|\mathbf{r}' - \mathbf{r}|^2}{2R_0^2}\right) / (2\pi R_0^2) \rightarrow \delta(\mathbf{r}' - \mathbf{r})$  in the limit  $R_0 \rightarrow 0$ . In other words, we consider that the continuous transition switches to a discontinuous transition at the singular situation in which  $c$  approaches infinity as  $1/R_0^2 \rightarrow \infty$  preserving the constant  $c_{\text{col}}$ .

Furthermore, we confirm that the transition point of the local collision model of the previous study [6] is reproduced as a singular limit of our model. By using the asymptotic form  $\mathcal{I}f_0 \rightarrow \rho_0 R_0^2$  at  $R_0 \rightarrow 0$ , the damping rate  $\text{Re } \Lambda_1(\mathbf{0})$  in Eq. (S14) becomes

$$\text{Re } \Lambda_1(\mathbf{0}) = s(1 - 2\pi p_1) - 8\rho_0 c R_0^2 \left(2\pi \hat{p}_1 - \frac{2}{3}\right), \quad (\text{S25})$$

and then we substitute  $c = c_{\text{col}}/(2\pi R_0^2)$

$$\text{Re } \Lambda_1(\mathbf{0}) = s(1 - 2\pi p_1) - \frac{8}{\pi} \rho_0 \frac{c_{\text{col}}}{2} \left(2\pi \hat{p}_1 - \frac{2}{3}\right), \quad (\text{S26})$$

We replace the notation as  $s \rightarrow \lambda$ ,  $c_{\text{col}} \rightarrow 2d_0 v_0$  and use the wrapped Gaussian distribution for the probability distributions  $p(\theta) = \sum_{n=-\infty}^{\infty} \frac{1}{\sqrt{2\pi}\sigma_0} \exp\left(-\frac{(\theta+2\pi n)^2}{2\sigma_0^2}\right)$  and  $\hat{p}(\theta) = \sum_{n=-\infty}^{\infty} \frac{1}{\sqrt{2\pi}\sigma} \exp\left(-\frac{(\theta+2\pi n)^2}{2\sigma^2}\right)$  as in Ref. [6], and then  $2\pi p_1 = e^{-\sigma_0^2/2}$ ,  $2\pi \hat{p}_1 = e^{-\sigma^2/2}$ . Thus, we get

$$\text{Re } \Lambda_1(\mathbf{0}) = \lambda \left(1 - e^{-\sigma_0^2/2}\right) - \frac{8}{\pi} \rho_0 d_0 v_0 \left(e^{-\sigma^2/2} - \frac{2}{3}\right), \quad (\text{S27})$$

This agrees with the coefficient  $-\mu$  in Eq. (31) in Ref. [6]. In addition, we get the transition density via  $\text{Re } \Lambda_1(\mathbf{0}) = 0$  (or  $\mu = 0$ ):

$$\rho_{0,\text{tr}} = \frac{\pi\lambda}{8d_0 v_0} \frac{1 - e^{-\frac{\sigma_0^2}{2}}}{e^{-\frac{\sigma^2}{2}} - \frac{2}{3}}. \quad (\text{S28})$$

This is equivalent to Eq. (35) in Ref. [6].

- 
- [1] D. Pita, B. A. Moore, L. P. Tyrrell, and E. Fernández-Juricic, PeerJ **3**, e1113 (2015).
  - [2] D. S. Calovi, A. Litchinko, V. Lecheval, U. Lopez, A. P. Escudero, H. Chaté, C. Sire, and G. Theraulaz, PLOS Comput. Biol. **14**, e1005933 (2018).
  - [3] B. Collignon, A. Séguret, and J. Halloy, R. Soc. open sci. **3**, 150473 (2016).
  - [4] R. Bainbridge, J. Exp. Biol. **35**, 109 (1958).
  - [5] O. Akanyeti, J. Putney, Y. R. Yanagitsuru, G. V. Lauder, W. J. Stewart, and J. C. Liao, Proc. Natl. Acad. Sci. U. S. A. **114**, 13828 (2017).
  - [6] E. Bertin, M. Droz, and G. Grégoire, J. Phys. A: Math. Theor. **42**, 445001 (2009).
